# Supplementary material for: A surgical system for automatic registration, stiffness mapping and dynamic image overlay
Source: arXiv:1711.08828 source file (2017-11-23)
Supplement: Supplementary file 1 [file additional.tex]

\section{Ease of Use}

\subsection{Maintaining the Integrity of the Specifications}

The IEEEtran class file is used to format your paper and style the text. All margins, 
column widths, line spaces, and text fonts are prescribed; please do not 
alter them. You may note peculiarities. For example, the head margin
measures proportionately more than is customary. This measurement 
and others are deliberate, using specifications that anticipate your paper 
as one part of the entire proceedings, and not as an independent document. 
Please do not revise any of the current designations.

\section{Prepare Your Paper Before Styling}
Before you begin to format your paper, first write and save the content as a 
separate text file. Complete all content and organizational editing before 
formatting. Please note sections \ref{AA}--\ref{SCM} below for more information on 
proofreading, spelling and grammar.

Keep your text and graphic files separate until after the text has been 
formatted and styled. Do not number text heads---{\LaTeX} will do that 
for you.

\subsection{Abbreviations and Acronyms}\label{AA}
Define abbreviations and acronyms the first time they are used in the text, 
even after they have been defined in the abstract. Abbreviations such as 
IEEE, SI, MKS, CGS, ac, dc, and rms do not have to be defined. Do not use 
abbreviations in the title or heads unless they are unavoidable.

\subsection{Units}
\begin{itemize}
\item Use either SI (MKS) or CGS as primary units. (SI units are encouraged.) English units may be used as secondary units (in parentheses). An exception would be the use of English units as identifiers in trade, such as ``3.5-inch disk drive''.
\item Avoid combining SI and CGS units, such as current in amperes and magnetic field in oersteds. This often leads to confusion because equations do not balance dimensionally. If you must use mixed units, clearly state the units for each quantity that you use in an equation.
\item Do not mix complete spellings and abbreviations of units: ``Wb/m\textsuperscript{2}'' or ``webers per square meter'', not ``webers/m\textsuperscript{2}''. Spell out units when they appear in text: ``. . . a few henries'', not ``. . . a few H''.
\item Use a zero before decimal points: ``0.25'', not ``.25''. Use ``cm\textsuperscript{3}'', not ``cc''.)
\end{itemize}

\subsection{Equations}
Number equations consecutively. To make your 
equations more compact, you may use the solidus (~/~), the exp function, or 
appropriate exponents. Italicize Roman symbols for quantities and variables, 
but not Greek symbols. Use a long dash rather than a hyphen for a minus 
sign. Punctuate equations with commas or periods when they are part of a 
sentence, as in:
\begin{equation}
a+b=\gamma\label{eq}
\end{equation}

Be sure that the 
symbols in your equation have been defined before or immediately following 
the equation. Use ``\eqref{eq}'', not ``Eq.~\eqref{eq}'' or ``equation \eqref{eq}'', except at 
the beginning of a sentence: ``Equation \eqref{eq} is . . .''

\subsection{\LaTeX-Specific Advice}

Please use ``soft'' (e.g., \verb|\eqref{Eq}|) cross references instead
of ``hard'' references (e.g., \verb|(1)|). That will make it possible
to combine sections, add equations, or change the order of figures or
citations without having to go through the file line by line.

Please don't use the \verb|{eqnarray}| equation environment. Use
\verb|{align}| or \verb|{IEEEeqnarray}| instead. The \verb|{eqnarray}|
environment leaves unsightly spaces around relation symbols.

Please note that the \verb|{subequations}| environment in {\LaTeX}
will increment the main equation counter even when there are no
equation numbers displayed. If you forget that, you might write an
article in which the equation numbers skip from (17) to (20), causing
the copy editors to wonder if you've discovered a new method of
counting.

{\BibTeX} does not work by magic. It doesn't get the bibliographic
data from thin air but from .bib files. If you use {\BibTeX} to produce a
bibliography you must send the .bib files. 

{\LaTeX} can't read your mind. If you assign the same label to a
subsubsection and a table, you might find that Table I has been cross
referenced as Table IV-B3. 

{\LaTeX} does not have precognitive abilities. If you put a
\verb|\label| command before the command that updates the counter it's
supposed to be using, the label will pick up the last counter to be
cross referenced instead. In particular, a \verb|\label| command
should not go before the caption of a figure or a table.

Do not use \verb|\nonumber| inside the \verb|{array}| environment. It
will not stop equation numbers inside \verb|{array}| (there won't be
any anyway) and it might stop a wanted equation number in the
surrounding equation.

\subsection{Some Common Mistakes}\label{SCM}
\begin{itemize}
\item The word ``data'' is plural, not singular.
\item The subscript for the permeability of vacuum $\mu_{0}$, and other common scientific constants, is zero with subscript formatting, not a lowercase letter ``o''.
\item In American English, commas, semicolons, periods, question and exclamation marks are located within quotation marks only when a complete thought or name is cited, such as a title or full quotation. When quotation marks are used, instead of a bold or italic typeface, to highlight a word or phrase, punctuation should appear outside of the quotation marks. A parenthetical phrase or statement at the end of a sentence is punctuated outside of the closing parenthesis (like this). (A parenthetical sentence is punctuated within the parentheses.)
\item A graph within a graph is an ``inset'', not an ``insert''. The word alternatively is preferred to the word ``alternately'' (unless you really mean something that alternates).
\item Do not use the word ``essentially'' to mean ``approximately'' or ``effectively''.
\item In your paper title, if the words ``that uses'' can accurately replace the word ``using'', capitalize the ``u''; if not, keep using lower-cased.
\item Be aware of the different meanings of the homophones ``affect'' and ``effect'', ``complement'' and ``compliment'', ``discreet'' and ``discrete'', ``principal'' and ``principle''.
\item Do not confuse ``imply'' and ``infer''.
\item The prefix ``non'' is not a word; it should be joined to the word it modifies, usually without a hyphen.
\item There is no period after the ``et'' in the Latin abbreviation ``et al.''.
\item The abbreviation ``i.e.'' means ``that is'', and the abbreviation ``e.g.'' means ``for example''.
\end{itemize}
An excellent style manual for science writers is \cite{b7}.

\subsection{Authors and Affiliations}
\textbf{The class file is designed for, but not limited to, six authors.} A 
minimum of one author is required for all conference articles. Author names 
should be listed starting from left to right and then moving down to the 
next line. This is the author sequence that will be used in future citations 
and by indexing services. Names should not be listed in columns nor group by 
affiliation. Please keep your affiliations as succinct as possible (for 
example, do not differentiate among departments of the same organization).

\subsection{Identify the Headings}
Headings, or heads, are organizational devices that guide the reader through 
your paper. There are two types: component heads and text heads.

Component heads identify the different components of your paper and are not 
topically subordinate to each other. Examples include Acknowledgments and 
References and, for these, the correct style to use is ``Heading 5''. Use 
``figure caption'' for your Figure captions, and ``table head'' for your 
table title. Run-in heads, such as ``Abstract'', will require you to apply a 
style (in this case, italic) in addition to the style provided by the drop 
down menu to differentiate the head from the text.

Text heads organize the topics on a relational, hierarchical basis. For 
example, the paper title is the primary text head because all subsequent 
material relates and elaborates on this one topic. If there are two or more 
sub-topics, the next level head (uppercase Roman numerals) should be used 
and, conversely, if there are not at least two sub-topics, then no subheads 
should be introduced.

\subsection{Figures and Tables}
\paragraph{Positioning Figures and Tables} Place figures and tables at the top and 
bottom of columns. Avoid placing them in the middle of columns. Large 
figures and tables may span across both columns. Figure captions should be 
below the figures; table heads should appear above the tables. Insert 
figures and tables after they are cited in the text. Use the abbreviation 
``Fig.~\ref{fig}'', even at the beginning of a sentence.

\begin{table}[htbp]
\caption{Table Type Styles}
\begin{center}
\begin{tabular}{|c|c|c|c|}
\hline
\textbf{Table}&\multicolumn{3}{|c|}{\textbf{Table Column Head}} \\
\cline{2-4} 
\textbf{Head} & \textbf{\textit{Table column subhead}}& \textbf{\textit{Subhead}}& \textbf{\textit{Subhead}} \\
\hline
copy& More table copy$^{\mathrm{a}}$& &  \\
\hline
\multicolumn{4}{l}{$^{\mathrm{a}}$Sample of a Table footnote.}
\end{tabular}
\label{tab1}
\end{center}
\end{table}
%
%\begin{figure}[htbp]
%\centerline{\includegraphics{fig1.png}}
%\caption{Example of a figure caption.}
%\label{fig}
%\end{figure}

Figure Labels: Use 8 point Times New Roman for Figure labels. Use words 
rather than symbols or abbreviations when writing Figure axis labels to 
avoid confusing the reader. As an example, write the quantity 
``Magnetization'', or ``Magnetization, M'', not just ``M''. If including 
units in the label, present them within parentheses. Do not label axes only 
with units. In the example, write ``Magnetization (A/m)'' or ``Magnetization 
\{A[m(1)]\}'', not just ``A/m''. Do not label axes with a ratio of 
quantities and units. For example, write ``Temperature (K)'', not 
``Temperature/K''.
